# Supplementary material for: Using Large Language Models to Generate JUnit Tests: An Empirical Study
Source: arXiv:2305.00418 source file (2024-03-09)
Supplement: Supplementary file 1 [file appendix.tex]

\appendices

  \section{Evosuite Project List}
  Source and details about the project can be found here: \url{https://www.evosuite.org/experimental-data/sf110/}. We used 47 projects in our study. In table \ref{tab:project}, we provided the name of the projects.
\begin{table}[ht!]
\centering\scriptsize
\caption{Project List from Evosuite Benchmark}
\label{tab:project}
\resizebox{\columnwidth}{!}{%
\begin{tabular}{|l|l|l|l|l|}
\hline
\textbf{Project Name} & \textbf{Project Name} & \textbf{Project Name} & \textbf{Project Name} & \textbf{Project Name} \\ \hline
a4j                   & inspirento            & diffi                 & objectexplorer        & ipcalculator          \\ \hline
rif                   & jmca                  & follow                & jtailgui              & classviewer           \\ \hline
templateit            & byuic                 & asphodel              & gae-app-manager       & quickserver           \\ \hline
jnfe                  & saxpath               & lilith                & biblestudy            & jclo                  \\ \hline
sfmis                 & jni-inchi             & dvd-homevideo         & lhamacaw              & heal                  \\ \hline
gfarcegestionfa       & apbsmem               & diebierse             & ext4j                 & jgaap                 \\ \hline
water-simulator       & xisemele              & lagoon                & fim1                  & sweethome3d           \\ \hline
imsmart               & httpanalyzer          & jhandballmoves        & fixsuite              &                       \\ \hline
dsachat               & javaviewcontrol       & mygrid                & openhre               &                       \\ \hline
omjstate              & sbmlreader2           & sugar                 & javathena             &                       \\ \hline
\end{tabular}%
}
\end{table}

\section{Test Smell List}
In Table \ref{tab:test-smell}, there is a list of test smells and their descriptions we considered in our work.
\begin{table}[ht!]
\centering\scriptsize
\caption{Test Smells Detectable by \textsc{TsDetect}~\cite{peruma2020tsdetect}}
\label{tab:test-smell}
\setlength{\tabcolsep}{1pt}
\begin{tabular}{@{}lp{5.6cm}@{}}
\toprule
\multicolumn{1}{c}{\textbf{\textbf{Test Smell}}} & \multicolumn{1}{c}{\textbf{\textbf{Description}}}                                                                                   \\ \midrule
Assertion Roulette (AR)                          & Multiple unexplained assertions in the same test method~\cite{Simula.SE.525}                                                        \\
Constructor Initialization (CI)                  & Test class with constructor method and field initialization~\cite{peruma19}                                                         \\
Conditional Logic Test (CLT)                     & Test methods that contain conditional statements~\cite{meszaros03}                                                                  \\
Duplicate Assert (DA)                            & More than one of the same verification method that checks the same parameters~\cite{peruma19}                                       \\
Default Test (DT)                                & Automatically generated test class with default name~\cite{peruma19}                                                                \\
Dependent Test (DPT)                                & Test being executed depends on other tests’ success\cite{peruma19}                                                              \\
Eager Test (EA)                                  & Test method that checks many methods of the object to be tested~\cite{Simula.SE.525}     \\
Exception Handling (EH)                          & When an exception handling is performed within a test method~\cite{peruma19}                                                        \\
Empty Test (EM)                                  & Test method without executable statements~\cite{peruma19}                                                                           \\
General Fixture (GF)                             & Setup method fields that are not used in all test methods~\cite{Simula.SE.525}           \\
Ignored Test (IT)                                & When a test method is ignored through the framework's annotation~\cite{peruma19}                                                    \\
Lazy Test (LT)                                   & Several test methods that verify the same production method~\cite{Simula.SE.525}         \\
Mystery Guest (MG)                               & When a test method uses and depends on external resources~\cite{Simula.SE.525}          \\
Magic Number Test (MNT)                          & Test Method that contains some number without indicating their purpose~\cite{meszaros03} \\
Redundant Assertion (RA)                         & Test method with checks that always have the same response~\cite{peruma19}                                                          \\
Resource Optimism (RO)                           & Test method that optimistically assumes the state of an external resource as available                                              \\
Redundant Print (RP)                             & Test method containing screen print statements~\cite{peruma19}                                                                      \\
Sensitive Equality (SE)                          & Use toString method in a test method to make validations~\cite{Simula.SE.525}            \\
Sleepy Test (ST)                                 & Test method with pauses to wait for an event~\cite{peruma19}                                                                        \\
Unknown Test (UT)                                & Test method without assertion~\cite{peruma19}                                                                                       \\
Verbose Test (VT)                                & Test method with many lines of code~\cite{meszaros03}                                    \\ \bottomrule
\end{tabular}
\end{table}

\section{Example Prompt Template}
\subsection{HumanEval}
In Listing \ref{lst:class_java}, a class under test is used in the RQ1, and in Listing \ref{lst:test_class_java}, there is a generated test class for this class under test. The highlighted part in Listing \ref{lst:test_class_java} is part of the prompt.
\begin{listing}[!ht]
{\renewcommand\theFancyVerbLine{%
\rmfamily\tiny\ifnum\value{FancyVerbLine}=25
  \setcounter{FancyVerbLine}{32}\ldots
\else
\arabic{FancyVerbLine}%
\fi
}
\begin{JavaSourceCode*}{label=\textcolor{black}{\tiny{TriangleArea.java}}}
package original;

class TriangleArea {
    /**
     * Given length of a side and high return 
     * area for a triangle.
     *
     * > triangleArea(5, 3)
     * 7.5
     * > triangleArea(2, 2)
     * 2.0
     * > triangleArea(10, 8)
     * 40.0
     */
    public static Double triangleArea(int a, int h) {
        return (a * h) / 2.0;
    }
}
\end{JavaSourceCode*}
}
\caption{Class Under Test from HumanEval}\label{lst:class_java}
\end{listing}
\begin{listing}[!ht]
{\renewcommand\theFancyVerbLine{%
\rmfamily\tiny\ifnum\value{FancyVerbLine}=25
  \setcounter{FancyVerbLine}{32}\ldots
\else
\arabic{FancyVerbLine}%
\fi
}
\begin{JavaSourceCode*}{label=\textcolor{black}{\tiny{TriangleAreaTest.java}},highlightlines={1-9}}
// TriangleAreaTest.java
package original;

import java.util.Arrays;
import java.util.Map;
import org.junit.jupiter.api.Test;
import static org.junit.jupiter.api.Assertions.*;

class TriangleAreaTest {
    @Test
	public void test1() throws Exception {
		assertEquals(7.5, original
                    .TriangleArea.triangleArea(5, 3));
	}

	@Test
	public void test2() throws Exception {
		assertEquals(2.0, original
                    .TriangleArea.triangleArea(2, 2));
	}

	@Test
	public void test3() throws Exception {
		assertEquals(40.0, original
                    .TriangleArea.triangleArea(10, 8));
	}
}
\end{JavaSourceCode*}
}
\caption{Test Class for Class Under Test from HumanEval}\label{lst:test_class_java}
\end{listing}

\subsection{Evosuite SF110 Benchmark}
In Listing \ref{lst:class_java_sf110}, there is a class under test taken from \textit{\textbf{jhandballmoves}} project used in the RQ1. However, for a better presentation, we remove other class contents. We only keep the class under test, the method under test, and its JavaDoc.
In Listing \ref{lst:test_class_java_sf110}, there is a generated test class for this method under the test of the class under test. The highlighted part in Listing \ref{lst:test_class_java_sf110} is part of the prompt.

\begin{listing}[!ht]
{\renewcommand\theFancyVerbLine{%
\rmfamily\tiny\ifnum\value{FancyVerbLine}=25
  \setcounter{FancyVerbLine}{32}\ldots
\else
\arabic{FancyVerbLine}%
\fi
}
\begin{JavaSourceCode*}{label=\textcolor{black}{\tiny{JMenuHelper.java}}}
package visu.handball.moves.controller;

import java.awt.event.*;
import javax.swing.*;

public class JMenuHelper {
/**
	 * Add an element to the menubar.
	 * 
	 * @param menuBar a JMenuBar
	 * @param s a String
	 * 
	 * @return added JMenu
	 */
	public static JMenu addMenuBarItem(JMenuBar menuBar, String s) {
		JMenu menu;

		/**
		 * Suche nach '_' und nimm das nächste Zeichen als Mnemonic,
		 * sonst: normales Menu
		 */
		if (s.indexOf("_") > -1) {
			int pos = s.indexOf("_");
			char c = s.charAt(pos + 1);
			StringBuffer sb = new StringBuffer(s).delete(pos, pos + 1);
			menu = new JMenu(sb.toString());
			menu.setMnemonic(c);
		} else
			menu = new JMenu(s);

		menuBar.add(menu);
		return menu;
	}
 }
\end{JavaSourceCode*}
}
\caption{Class Under Test from Evosuite SF110 }\label{lst:class_java_sf110}
\end{listing}
\begin{listing}[!ht]
{\renewcommand\theFancyVerbLine{%
\rmfamily\tiny\ifnum\value{FancyVerbLine}=25
  \setcounter{FancyVerbLine}{32}\ldots
\else
\arabic{FancyVerbLine}%
\fi
}
\begin{JavaSourceCode*}{label=\textcolor{black}{\tiny{JMenuHelperTest.java}},highlightlines={1-15}}
// JMenuHelperTest.java
package visu.handball.moves.controller;

import java.awt.event.*;
import javax.swing.*;
import java.util.*;
import org.junit.jupiter.api.*;
import static org.junit.jupiter.api.Assertions.*;

/**
 * Test class of {@link JMenuHelper}.
 * It contains one unit test case for the 
 * {@link JMenuHelper#addMenuBarItem(JMenuBar, String)} method.
 */
class scenario3_JMenuHelper_addMenuBarItem_2000_10_Test {

    // Default Constructor
    scenario3_JMenuHelper_addMenuBarItem_2000_10_Test() {
        // Test code for a javax.swing component that implements event.
    }

    // Test methods for each of classes in this class.
    /**
     * Tests {@link JMenuHelper#addMenuBarItem(JMenuBar, String)}.
     */
    @Test
    public void testAddMenuItem() {
        assertNotSame(null, addMenuBarItem(null, ""));
        assertNotSame(null, addMenuBarItem(new JMenuBar(), ""));
        assertNotSame(null, addMenuBarItem("", ""));
    }
}
\end{JavaSourceCode*}
}
\caption{Test Class for Class Under Test from Evosuite SF110 }\label{lst:test_class_java_sf110}
\end{listing}
